# Supplementary material for: Classical-Nonclassical Polarity of Gaussian States
Source: arXiv:2310.12104 source file (2023-10-25)
Supplement: Supplementary file 1 [file Supplementary_for__Classical_Nonclassical_Polarity_of_Gaussian_States_.pdf]

# Supplementary for "Classical-Nonclassical Polarity of Gaussian States"


Jiru Liu,[1,*] Wenchao Ge,[2,†] and M. Suhail Zubairy[1,‡]

[1]Institute for Quantum Science and Engineering (IQSE) and Department of Physics and Astronomy, Texas A&M University, College Station, TX 77843-4242, USA

[2]Department of Physics, University of Rhode Island, Kingston, Rhode Island 02881, USA



(Dated: October 17, 2023)


## Contents


I. Single-mode nonclassicality depth of Gaussian states 1
- I.1. Gaussian states preliminary 1
- I.2. Nonclassicality depth 2

II. Symplectic invariants of Gaussian states 3

III. Symplectic invariants of PPT Gaussian state 4
- III.1. two-mode scenario 4
- III.2. three-mode scenario 5

IV. Beamsplitter (BS) operation 5

V. Derivation of total polarity for two-mode, three-mode Gaussian state 5
- V.1. two-mode scenario 5
- V.2. three-mode scenario 6

VI. Proof of theorem 2 6

References 7


## I. Single-mode nonclassicality depth of Gaussian states

### I.1. Gaussian states preliminary

An $n$-mode Gaussian state is defined as a state whose characteristic function $\chi(\boldsymbol{u})$ follows a Gaussian distribution, i.e.,

$$\chi(\boldsymbol{u}) = \mathrm{Tr}(e^{-i\boldsymbol{u}^\dagger\hat{\boldsymbol{r}}}\rho) = \exp(-\frac{1}{2}\boldsymbol{u}^\dagger\boldsymbol{\gamma}\boldsymbol{u} - i\boldsymbol{u}^\dagger\boldsymbol{d}), \tag{I.1}$$

where $\boldsymbol{u}^\dagger = [\alpha_1^*, \alpha_1, ...\alpha_n^*, \alpha_n]$ are the variables for the characteristic function, $\hat{\boldsymbol{r}} = [\hat{a}_1^\dagger, \hat{a}_1, ...\hat{a}_n^\dagger, \hat{a}_n]^\dagger$ is the vector of bonsic field operators. The coefficient matrix $\boldsymbol{\gamma}$ is called the covariance matrix (CM) while $\boldsymbol{d}$ is the displacing vector, where

$$\gamma_{jk} = \frac{1}{2}\langle \Delta\hat{\boldsymbol{r}}_j^\dagger \Delta\hat{\boldsymbol{r}}_k + \Delta\hat{\boldsymbol{r}}_k \Delta\hat{\boldsymbol{r}}_j^\dagger \rangle, \quad \boldsymbol{d}_j = \langle \hat{\boldsymbol{r}}_j \rangle. \tag{I.2}$$

Note that $\Delta\hat{\boldsymbol{r}}_j$ denotes $\hat{\boldsymbol{r}}_j - \langle\hat{\boldsymbol{r}}\rangle_j$, the bracket $\langle\hat{X}\rangle = \mathrm{Tr}(\rho\hat{X})$.

The displacing vector is a trivial parameter that represents the mean position of the state within the phase space. Given a single-mode Gaussian state in phase space, it is always possible to shift it to the zero point such that $\boldsymbol{d} = \boldsymbol{0}$. Consequently, the CM can be expressed as:

$$\boldsymbol{\gamma} = \begin{bmatrix} \frac{1}{2}\langle\hat{a}^\dagger\hat{a} + \hat{a}\hat{a}^\dagger\rangle & \langle\hat{a}^\dagger\hat{a}^\dagger\rangle \\ \langle\hat{a}\hat{a}\rangle & \frac{1}{2}\langle\hat{a}^\dagger\hat{a} + \hat{a}\hat{a}^\dagger\rangle \end{bmatrix} = \begin{bmatrix} a & b^* \\ b & a \end{bmatrix}. \tag{I.3}$$

---


* ljr1996@tamu.edu

† wenchao.ge@uri.edu

‡ zubairy@physics.tamu.edu

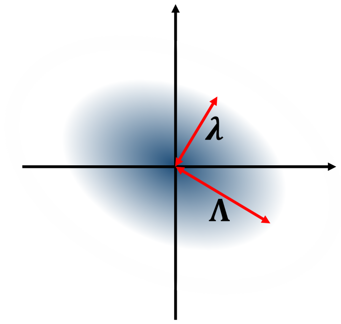


FIG. 1. A single-mode Gaussian state in phase space. $\lambda, \Lambda$ are the minimum and maximum uncertainties of the quadrature operators, respectively.

### I.2. Nonclassicality depth

The Sudarshan-Glauber $P$ representation of a single-mode state is given by [1]

$$\begin{aligned} P(\beta) &= \frac{1}{\pi^2}\int d^2\alpha \, \mathrm{Tr}(e^{-i\alpha^*\hat{a}-i\alpha\hat{a}^\dagger}\rho)e^{\frac{1}{2}|\alpha|^2}e^{i\alpha^*\beta+i\alpha\beta^*} \\ &= \frac{1}{\pi^2}\int d^2\alpha \, \chi(\alpha,\alpha^*)e^{\frac{1}{2}|\alpha|^2}e^{i\alpha^*\beta+i\alpha\beta^*} \end{aligned} \tag{I.4}$$

As a distribution function, $P$ is required to be positive definite. If it is not, the state is considered nonclassical. Building upon the $P$ function, another distribution function, the $R$ function, is defined as: [2]

$$R_\tau(\omega) = \frac{1}{\tau\pi}\int d^2\beta \, \exp(-\frac{1}{\tau}|\omega-\beta|^2)P(\beta). \tag{I.5}$$

The minimum value of $\tau$ for $R$ to be positive is defined the nonclassicality depth.

Substituting the expression of the $P$ function in Eq. (I.4) into Eq. (I.5):

$$\begin{aligned} R_\tau(\alpha) &= \frac{1}{\tau\pi}\int d^2\beta \, \exp(-\frac{1}{\tau}(|\omega|^2+|\beta|^2-\omega^*\beta-\omega\beta^*))\,\frac{1}{\pi^2}\int d^2\alpha \, \chi(\alpha^*,\alpha)e^{\frac{1}{2}|\alpha|^2}e^{i\alpha^*\beta+i\alpha\beta^*} \\ &= \frac{1}{\tau\pi^3}\int d^2\alpha \, \chi(\alpha^*,\alpha)e^{\frac{1}{2}|\alpha|^2-\frac{1}{\tau}|\omega|^2}\int d^2\beta \, \exp\left[-\frac{1}{\tau}|\beta|^2+(i\alpha+\frac{\omega}{\tau})\beta^*+(i\alpha^*+\frac{\omega^*}{\tau})\beta\right] \\ &= \frac{1}{\tau\pi^3}\int d^2\alpha \, \chi(\alpha^*,\alpha)e^{\frac{1}{2}|\alpha|^2-\frac{1}{\tau}|\omega|^2}\pi\tau\exp\left[\tau(i\alpha+\frac{\omega}{\tau})(i\alpha^*+\frac{\omega^*}{\tau})\right] \\ &= \frac{1}{\pi^2}\int d^2\alpha \, \chi(\alpha^*,\alpha)\exp\left[(\frac{1}{2}-\tau)|\alpha|^2+i\alpha^*\omega+i\alpha\omega^*\right]. \end{aligned} \tag{I.6}$$

According to Eq. (I.1), $\chi(\alpha^*,\alpha) = \exp(-\frac{1}{2}\boldsymbol{u}^\dagger\boldsymbol{\gamma}\boldsymbol{u} - i\boldsymbol{u}^\dagger\boldsymbol{d})$, where $\boldsymbol{u}^\dagger = [\alpha^*,\alpha]$. For $R$ function to be positive and convergent, the integration over $\omega$ implies that $\boldsymbol{\gamma} \geqslant (1/2-\tau)$, hence $\tau \geqslant 1/2-\lambda$, where $\lambda$ is the minimum eigrnvalue of $\boldsymbol{\gamma}$. Hence, the nonclassicality depth is defined as $\tau_{\min}\max\{0, 1/2-\lambda\}$.

A single-mode Gaussian state $\rho$, in general, is a displaced squeezing thermal state, i.e. $\rho = \hat{D}\hat{S}\rho_{\mathrm{th}}\hat{S}^\dagger\hat{D}^\dagger$, where $\hat{S}(r,\phi) = \exp(re^{i\phi}\hat{a}^{\dagger 2} - re^{-i\phi}\hat{a}^2)$ is the squeezing operator, and $\hat{D}(\alpha) = \exp(\alpha\hat{a}^\dagger - \alpha^*\hat{a})$ is the displacing operator. The CM in this case is given by

$$\boldsymbol{\gamma} = \begin{bmatrix} \cosh r & e^{i\phi}\sinh r \\ e^{-i\phi}\sinh r & \cosh r \end{bmatrix}\begin{bmatrix} 1/2+\langle n_{\mathrm{th}}\rangle & 0 \\ 0 & 1/2+\langle n_{\mathrm{th}}\rangle \end{bmatrix}\begin{bmatrix} \cosh r & e^{i\phi}\sinh r \\ e^{-i\phi}\sinh r & \cosh r \end{bmatrix} = \left(\frac{1}{2}+\langle n_{\mathrm{th}}\rangle\right)\begin{bmatrix} \cosh 2r & e^{-i\phi}\sinh 2r \\ e^{i\phi}\sinh 2r & \cosh 2r \end{bmatrix} \tag{I.7}$$

The eigenvalues $\lambda = (1/2+\langle n_{\mathrm{th}}\rangle)e^{-2r}$, $\Lambda = (1/2+\langle n_{\mathrm{th}}\rangle)e^{2r}$ can be easily obtained from Eq. (I.7). Note that $\lambda, \Lambda$ represents the minimum and maximum variance of a pair of quadrature operators (see Fig. 1). According to nonclassicality depth $\tau_{\min} = \max\{0, 1/2-\lambda\}$, it can be seen that the average number of thermal photons, $\langle n_{\mathrm{th}}\rangle$, contributes to the classical character of the state, while the squeezing factor, $r$, contributes to its nonclassical features.

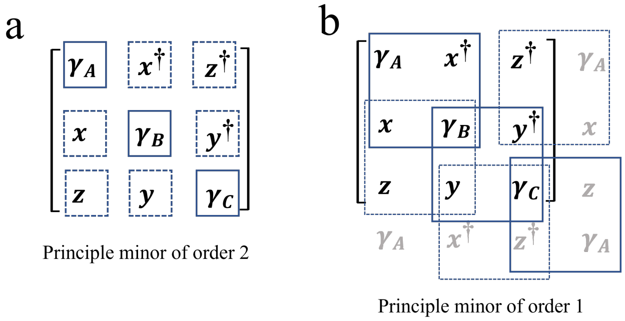


FIG. 2. **a.** $\mathcal{I}_2^{(3)}$ is the summation of determinant of all nine $2\times 2$ matrices in the rectangle. Solid rectangle means single-mode state CM while dashed one means interaction CM. **b.** $\mathcal{I}_1^{(2)}$ is the summation of the determinants of nine $4\times 4$ matrices. The solid rectangles represent $\gamma_{AB}$, $\gamma_{BC}$, and $\gamma_{AC}$, and the dashed rectangles denote the matrices $\boldsymbol{D_x}$, $\boldsymbol{D_y}$, and $\boldsymbol{D_z}$. Each rectangle is a $4\times 4$ matrices by taking one of the nine blocks as a vertex and expanding to a $2\times 2$ block to the right and to the bottom.

## II. Symplectic invariants of Gaussian states

Symplectic invariants are quantities derived from the covariance matrix (CM) of Gaussian states which exhibit an intriguing property: they remain unchanged under symplectic transformations applied to the CM. As previously discussed, any Gaussian unitary transformation applied to Gaussian states corresponds to a symplectic transformation. Consequently, symplectic invariants are inherently linked to conserved physical quantities. In the subsequent sections, we will illustrate their significant role in determining symplectic eigenvalues $\nu$, which are critical to entanglement.

In the case of a single-mode Gaussian state, a straightforward symplectic invariant is the determinant of the CM $\gamma^{(1)}$, denoted as $\mathcal{I}_0^{(1)} = |\gamma^{(1)}| = \nu^2$, where $\nu$ is the symplectic enigenvalue of $\gamma^{(1)}$.

For a two-modes Gaussian state, whose CM is denoted by $\gamma^{(2)}$, the two symplectic invariants are: 1) $\mathcal{I}_0^{(2)} = |\gamma^{(2)}| = \nu_1^2\nu_2^2$; 2) $\mathcal{I}_1^{(2)} = |\gamma_{\boldsymbol{A}}| + |\gamma_{\boldsymbol{B}}| + 2|\boldsymbol{x}| = \nu_1^2 + \nu_2^2$.

$$\gamma^{(2)} = \begin{bmatrix} \gamma_{\boldsymbol{A}} & \boldsymbol{x}^\dagger \\ \boldsymbol{x} & \gamma_{\boldsymbol{B}} \end{bmatrix} \tag{II.1}$$

For three-mode $\gamma^{(3)}$

$$\gamma^{(3)} = \begin{bmatrix} \gamma_{\boldsymbol{A}} & \boldsymbol{x}^\dagger & \boldsymbol{z}^\dagger \\ \boldsymbol{x} & \gamma_{\boldsymbol{B}} & \boldsymbol{y}^\dagger \\ \boldsymbol{z} & \boldsymbol{y} & \gamma_{\boldsymbol{C}} \end{bmatrix}, \tag{II.2}$$

The symplectic invariants of the three-mode Gaussian state are $\mathcal{I}_0^{(3)} = |\gamma_{\boldsymbol{ABC}}|$, $\mathcal{I}_1^{(3)} = |\gamma_{\boldsymbol{AB}}| + |\gamma_{\boldsymbol{BC}}| + |\gamma_{\boldsymbol{AC}}| + 2|\boldsymbol{D_x}| + 2|\boldsymbol{D_y}| + 2|\boldsymbol{D_z}|$, and $\mathcal{I}_2^{(3)} = |\gamma_{\boldsymbol{A}}| + |\gamma_{\boldsymbol{B}}| + |\gamma_{\boldsymbol{C}}| + 2|\boldsymbol{x}| + 2|\boldsymbol{y}| + 2|\boldsymbol{z}|$, where $\boldsymbol{D_x}, \boldsymbol{D_y}, \boldsymbol{D_z}$ are $4\times 4$ matrices given by:

$$\boldsymbol{D_x} = \begin{bmatrix} \boldsymbol{x} & \gamma_{\boldsymbol{B}} \\ \boldsymbol{z} & \boldsymbol{y} \end{bmatrix}, \quad \boldsymbol{D_y} = \begin{bmatrix} \boldsymbol{y} & \gamma_{\boldsymbol{C}} \\ \boldsymbol{x}^\dagger & \boldsymbol{z}^\dagger \end{bmatrix}, \quad \boldsymbol{D_z} = \begin{bmatrix} \boldsymbol{z} & \boldsymbol{y} \\ \gamma_{\boldsymbol{A}} & \boldsymbol{x}^\dagger \end{bmatrix}. \tag{II.3}$$

The pattern of $\mathcal{I}_2^{(3)}$ and $\mathcal{I}_2^{(3)}$ are explained in Fig. 2. Note that $|\boldsymbol{D_x}|$ is the second order minor after deleting the first row and the third column of blocked $\gamma_{\boldsymbol{ABC}}$, $|\boldsymbol{D_y}|$ is the second order minor after deleting the second row and the first column, $|\boldsymbol{D_z}|$ is the second order minor after deleting the second row and the third column. Also note that $|\boldsymbol{D_x}| = |\boldsymbol{D_{x^\dagger}}|$, $|\boldsymbol{D_y}| = |\boldsymbol{D_{y^\dagger}}|$, and $|\boldsymbol{D_z}| = |\boldsymbol{D_{z^\dagger}}|$.

According to Ref. [3, 4], together with the case of single-mode and two-mode state symplectic invariants, we conclude that

**Theorem II.1** *For a n-mode Gaussian state whose CM is the blocked matrix $\gamma^{(n)}$, $\gamma^{(n)}$ consists of $n\times n$ elements, each elements is a $2\times 2$ matrix representing reduced single-mode state or correlation matrix of two modes. There are n symplectic invariants $\{\mathcal{I}_0, ...\mathcal{I}_{n-1}\}$ given by*

$$\mathcal{I}_k^{(n)} = \sum \mathcal{M}_{n-k}(\gamma^{(n)}). \tag{II.4}$$

*Here, $\mathcal{M}_{n-k}(\gamma^{(n)})$ denotes the minor of order $n-k$ of the blocked matrix $\gamma^{(n)}$. The summation runs over all possible $(n-k)$th order minors.*

To preempt any possible confusion about the above theorem, we explain by adding a few points as following:

(1). The minor of order $n-k$ of a matrix $\boldsymbol{A}$ is obtained by deleting $k$ rows and $k$ columns from $\boldsymbol{A}$, then calculating the determinant of the remaining matrix. Taking $\boldsymbol{A} = \begin{bmatrix} a & b \\ b & c \end{bmatrix}$ for example, the order 2 minor is $\mathcal{M}_2(\boldsymbol{A}) = ac - b^2$, while order 1 minor $\mathcal{M}_1(\boldsymbol{A})$ has four values: $c$ (deleting the first row and first column); $b$ (deleting the first row, second column or deleting the second row, first column); $a$ (deleting the second row, second column). Thus, $\sum \mathcal{M}_1(\boldsymbol{A}) = a + c + 2b$.

(2). The minor is for the blocked form of $\gamma^{(n)}$, in which context deleting one row or one columns of blocked $\gamma^{(n)}$ means deleting two rows or two columns of $2n \times 2n$ $\gamma^{(n)}$. For example, a two-mode Gaussian state CM given by Eq.(II.1), the invariants $\mathcal{I}_1^{(2)}$ is given by

$$\mathcal{I}_1^{(2)} = \sum \mathcal{M}_{2-1}(\gamma^{(2)}) = |\gamma_{\boldsymbol{A}}| + |\gamma_{\boldsymbol{B}}| + 2|\boldsymbol{x}|. \tag{II.5}$$

(3). The number of terms in minor of order $k$ is calculated by $\binom{n}{k} \times \binom{n}{k}$. According to Williamson's theorem [5], the CM $\gamma^{(n)}$ can always be symplectic diagonalized to $\mathrm{diag}(\nu_1, \nu_1, \nu_2, \nu_2, \cdots, \nu_n, \nu_n)$. Here $\nu_j$ are the symplectic eigenvalues. By calculating the symplectic invariants of the diagonalized matrix, one can find that

**Theorem II.2** *The symplectic invariants* $\{\mathcal{I}_0^{(n)}, ...\mathcal{I}_{n-1}^{(n)}\}$ *are connected to symplectic invariants* $\{\nu_i\}$ *by*

$$\begin{aligned}
\mathcal{I}_0^{(n)} &= \nu_1^2 \nu_2^2 ... \nu_n^2 \\
\mathcal{I}_1^{(n)} &= \nu_2^2 ... \nu_n^2 + \nu_1^2 \nu_3^2 ... \nu_n^2 + ... \nu_1^2 ... \nu_{n-1}^2 \\
\mathcal{I}_2^{(n)} &= \nu_3^2 ... \nu_n^2 + \nu_2^2 \nu_4^2 ... \nu_n^2 + ... \nu_1^2 ... \nu_{n-2}^2 \\
&\vdots \\
\mathcal{I}_{n-1}^{(n)} &= \nu_1^2 + \nu_2^2 + ... + \nu_n^2
\end{aligned} \tag{II.6}$$

*A concise, mathematical expression of the above theorem is*

$$\mathcal{I}_k^{(n)} = \sum_{\mathcal{S}_k^n} \prod_{j \in \mathcal{S}_k^n} \nu_j^2, \tag{II.7}$$

*where* $\mathcal{S}_k^n$ *represents a subset of* $n-k$ *integers chosen from integers* $1, 2, ..., n$ *and the summation goes over all possible subsets.*

## III. Symplectic invariants of PPT Gaussian state

### III.1. two-mode scenario

According to the last section, the symplectic invariants for two-mode Gaussian states $\rho_{AB}$, whose CM is given by Eq. (II.1), are

$$\begin{aligned}
\nu_A^2 + \nu_B^2 &= \mathcal{I}_1^{(2)} = |\gamma_{\boldsymbol{A}}| + |\gamma_{\boldsymbol{B}}| + 2|\boldsymbol{x}| \\
\nu_A^2 \nu_B^2 &= \mathcal{I}_0^{(2)} = |\gamma_{\boldsymbol{AB}}|
\end{aligned} \tag{III.1}$$

Positive partial transpose (PPT) theory is a powerful tool in determining Gaussian state entanglement. A two-mode Gaussian state are entangled if and only if it is not positive partial transpose (NPPT) state [6–8]. , Denote the PPT state $\rho_{AB}^{T_A}$ as $\tilde{\rho}_{AB}$ (take partial transpose of mode $A$ for instance), the CM of $\tilde{\rho}_{AB}$, which is denoted as $\tilde{\gamma}_{\boldsymbol{AB}}$, can be easily obtained as [8]

$$\tilde{\gamma}_{\boldsymbol{AB}} = \begin{bmatrix} \boldsymbol{t} & \boldsymbol{0} \\ \boldsymbol{0} & \mathbb{1} \end{bmatrix} \begin{bmatrix} \gamma_{\boldsymbol{A}} & \boldsymbol{x}^\dagger \\ \boldsymbol{x} & \gamma_{\boldsymbol{B}} \end{bmatrix} \begin{bmatrix} \boldsymbol{t} & \boldsymbol{0} \\ \boldsymbol{0} & \mathbb{1} \end{bmatrix} = \begin{bmatrix} \boldsymbol{t}\gamma_{\boldsymbol{A}}\boldsymbol{t} & \boldsymbol{t}\boldsymbol{x}^\dagger \\ \boldsymbol{x}\boldsymbol{t} & \gamma_{\boldsymbol{B}} \end{bmatrix}, \qquad \boldsymbol{t} = \begin{bmatrix} 0 & 1 \\ 1 & 0 \end{bmatrix} \tag{III.2}$$

Following the methods utilized in Eq. (III.1), the symplectic invariants of PPT state $\tilde{\gamma}_{\boldsymbol{AB}}$, denoted as $\tilde{\mathcal{I}}_0^{(2)}, \tilde{\mathcal{I}}_1^{(2)}$, are calculated by

$$\begin{aligned}
\tilde{\nu}_A^2 + \tilde{\nu}_B^2 &= \tilde{\mathcal{I}}_1^{(2)} = |\boldsymbol{t}\gamma_{\boldsymbol{A}}\boldsymbol{t}| + |\gamma_{\boldsymbol{B}}| + 2|\boldsymbol{x}\boldsymbol{t}| = |\gamma_{\boldsymbol{A}}| + |\gamma_{\boldsymbol{B}}| - 2|\boldsymbol{x}| = \mathcal{I}_1^{(2)} - 4|\boldsymbol{x}| \\
\tilde{\nu}_A^2 \tilde{\nu}_B^2 &= \tilde{\mathcal{I}}_0^{(2)} = |\tilde{\gamma}_{\boldsymbol{AB}}| = |\gamma_{\boldsymbol{AB}}| = \mathcal{I}_0^{(2)}
\end{aligned} \tag{III.3}$$

Note that $|\boldsymbol{t}| = 1$. $\tilde{\nu}_A$ and $\tilde{\nu}_B$ are the sympletic eigenvalues of $\tilde{\gamma}_{\boldsymbol{ABC}}$. Using $|\boldsymbol{t}| = -1$, the relation between $\mathcal{I}_0, \mathcal{I}_1$ and $\tilde{\mathcal{I}}_0, \tilde{\mathcal{I}}_1$ can be obtained as shown by Eq. (III.3).

### III.2. three-mode scenario

The CM of $\rho_{ABC}^{T_A}$, denoted as $\tilde{\gamma}_{\boldsymbol{ABC}}$, can be obtained using the same methods of Eq. (III.2),

$$\tilde{\gamma}_{\boldsymbol{ABC}} = \begin{bmatrix} \boldsymbol{t}\boldsymbol{\gamma_A}\boldsymbol{t} & \boldsymbol{t}\boldsymbol{x}^\dagger & \boldsymbol{t}\boldsymbol{z}^\dagger \\ \boldsymbol{x}\boldsymbol{t} & \boldsymbol{\gamma_B} & \boldsymbol{y}^\dagger \\ \boldsymbol{z}\boldsymbol{t} & \boldsymbol{y} & \boldsymbol{\gamma_C} \end{bmatrix}, \tag{III.4}$$

The symplectic invariants of $\tilde{\gamma}_{\boldsymbol{ABC}}$, are given by

$$\begin{aligned} \tilde{\nu}_A^2\tilde{\nu}_B^2\tilde{\nu}_C^2 &= \tilde{I}_0^{(3)} = I_0^{(3)} \\ \tilde{\nu}_A^2\tilde{\nu}_B^2 + \tilde{\nu}_B^2\tilde{\nu}_C^2 + \tilde{\nu}_A^2\tilde{\nu}_C^2 &= \tilde{I}_1^{(3)} = I_1^{(3)} - 4|\boldsymbol{D_x}| - 4|\boldsymbol{D_y}| \\ \tilde{\nu}_A^2 + \tilde{\nu}_B^2 + \tilde{\nu}_C^2 &= \tilde{I}_2^{(3)} = I_2^{(3)} - 4|\boldsymbol{x}| - 4|\boldsymbol{z}|. \end{aligned} \tag{III.5}$$

## IV. Beamsplitter (BS) operation

In general, consider a two-mode Gaussian state mixed by a beamsplitter $BS(\theta,\varphi)$. Take the input state CM $\boldsymbol{\gamma_{AB}}$ as the most general form introduced by Eq. (II.1). The beamsplitter symplectic operation $\boldsymbol{S}_{BS}(\theta,\varphi)$ is given by:

$$\boldsymbol{S}_{BS} = \begin{bmatrix} \cos\theta\,\mathbb{1}_2 & \sin\theta\,\boldsymbol{\varphi} \\ -\sin\theta\,\boldsymbol{\varphi}^\dagger & \cos\theta\,\mathbb{1}_2 \end{bmatrix}, \quad \boldsymbol{\varphi} = \begin{bmatrix} e^{i\varphi} & 0 \\ 0 & e^{-i\varphi} \end{bmatrix}. \tag{IV.1}$$

After applying the beam-splitter operation, the output state CM is transformed as:

$$\boldsymbol{\gamma_{A'B'}} = \boldsymbol{S}_{BS}\boldsymbol{\gamma_{AB}}\boldsymbol{S}_{BS}^\dagger = \begin{bmatrix} \boldsymbol{\gamma_{A'}} & \boldsymbol{x'}^\dagger \\ \boldsymbol{x'} & \boldsymbol{\gamma_{B'}} \end{bmatrix} \tag{IV.2}$$

where

$$\begin{aligned} \boldsymbol{\gamma_{A'}} &= \cos^2\theta\,\boldsymbol{\gamma_A} + \sin^2\theta\,\boldsymbol{\varphi}\boldsymbol{\gamma_B}\boldsymbol{\varphi}^\dagger + \sin\theta\cos\theta\,(\boldsymbol{\varphi}\boldsymbol{x} + \boldsymbol{x}^\dagger\boldsymbol{\varphi}^\dagger) \\ \boldsymbol{\gamma_{B'}} &= \cos^2\theta\,\boldsymbol{\gamma_B} + \sin^2\theta\,\boldsymbol{\varphi}^\dagger\boldsymbol{\gamma_A}\boldsymbol{\varphi} - \sin\theta\cos\theta\,(\boldsymbol{x}\boldsymbol{\varphi} + \boldsymbol{\varphi}^\dagger\boldsymbol{x}^\dagger) \\ \boldsymbol{x'} &= \sin\theta\cos\theta\,(\boldsymbol{\gamma_B}\boldsymbol{\varphi}^\dagger - \boldsymbol{\varphi}^\dagger\boldsymbol{\gamma_A}) + \cos^2\theta\,\boldsymbol{x} - \sin^2\theta\,\boldsymbol{\varphi}^\dagger\boldsymbol{x}^\dagger\boldsymbol{\varphi}^\dagger \end{aligned} \tag{IV.3}$$

Note that $\lambda_A + \Lambda_A = (\boldsymbol{\gamma_A})_{11} - |(\boldsymbol{\gamma_A})_{12}| + (\boldsymbol{\gamma_A})_{11} + |(\boldsymbol{\gamma_A})_{12}| = 2(\boldsymbol{\gamma_A})_{11}$, for the output state $\rho_{A'B'}$,

$$\begin{aligned} \lambda_{A'} + \Lambda_{A'} + \lambda_{B'} + \Lambda_{B'} &= 2\cos^2\theta\,(\boldsymbol{\gamma_A})_{11} + 2\sin^2\theta\,(\boldsymbol{\gamma_B})_{11} + 2\sin^2\theta\,(\boldsymbol{\gamma_A})_{11} + 2\cos^2\theta\,(\boldsymbol{\gamma_B})_{11} \\ &= 2(\boldsymbol{\gamma_A})_{11} + 2(\boldsymbol{\gamma_B})_{11} = \lambda_A + \Lambda_A + \lambda_B + \Lambda_B \end{aligned} \tag{IV.4}$$

For three mode scenario $\rho_{ABC}$, since the BS only involves two-mode operation, the same result can be obtained that

$$\lambda_{A'} + \Lambda_{A'} + \lambda_{B'} + \Lambda_{B'} + \lambda_{C'} + \Lambda_{C'} = \lambda_A + \Lambda_A + \lambda_B + \Lambda_B + \lambda_C + \Lambda_C \tag{IV.5}$$

## V. Derivation of total polarity for two-mode, three-mode Gaussian state

### V.1. two-mode scenario

In the main text Eq. (9), the total polarity $\mathcal{P}$ for two-mode Gaussian state $\rho_{AB}$ is given by

$$\mathcal{P} \equiv \mathcal{P}_A^{(1)} + \mathcal{P}_B^{(1)} + \mathcal{P}_{A:B}^{(2)} \tag{V.1}$$

According to Eq. (5) of the main text,

$$\begin{aligned} \mathcal{P}_A^{(1)} &= -(\lambda_A - \frac{1}{2})(\Lambda_A - \frac{1}{2}) \\ &= -|\boldsymbol{\gamma_A}| - \frac{1}{4} + \frac{1}{2}(\lambda_A + \Lambda_A) \end{aligned} \tag{V.2}$$

Hence, together with Eq. (7) of the main text,

$$\begin{aligned}\mathcal{P} &\equiv -|\gamma_{\boldsymbol{A}}| - |\gamma_{\boldsymbol{B}}| - \frac{1}{2} + \frac{1}{2}(\lambda_A + \Lambda_A + \lambda_B + \Lambda + B) - \frac{1}{8} + \frac{1}{2}\tilde{\mathcal{I}}_1^{(2)} - 2\tilde{\mathcal{I}}^{(2)} \\ &= \frac{1}{2}(\lambda_A + \Lambda_A + \lambda_B + \Lambda_B) + (-|\gamma_{\boldsymbol{A}}| - |\gamma_{\boldsymbol{B}}| + \frac{1}{2}|\gamma_{\boldsymbol{A}}| + \frac{1}{2}|\gamma_{\boldsymbol{B}}| - |\boldsymbol{x}|) - \frac{5}{8} - 2\mathcal{I}_0^{(2)} \\ &= \frac{1}{2}(\lambda_A + \Lambda_A + \lambda_B + \Lambda_B) - \frac{1}{2}\mathcal{I}_1^{(2)} - \frac{5}{8} - 2\mathcal{I}_0^{(2)}\end{aligned} \tag{V.3}$$

### V.2. three-mode scenario

In the main text Eq. (10), the total polarity $\mathcal{P}_T$ for three-mode Gaussian state $\rho_{ABC}$ is given by

$$\begin{aligned}\mathcal{P} &= \sum_{\alpha=A,B,C} \mathcal{P}_\alpha^{(1)} + \frac{1}{2}\sum_{\alpha,\beta=A,B,C} \mathcal{P}_{\alpha:\beta}^{(2)} + \frac{1}{2}\sum_{\alpha,\beta,\kappa=A,B,C} \mathcal{P}_{\alpha:\beta\kappa}^{(3)} \\ &= \mathcal{P}_A^{(1)} + \mathcal{P}_B^{(1)} + \mathcal{P}_C^{(1)} + \mathcal{P}_{AB}^{(2)} + \mathcal{P}_{BC}^{(2)} + \mathcal{P}_{CA}^{(2)} + \mathcal{P}_{A:BC}^{(3)} + \mathcal{P}_{B:AC}^{(3)} + \mathcal{P}_{C:AB}^{(3)}\end{aligned} \tag{V.4}$$

According to Eq. (7) of the main text,

$$\begin{aligned}\mathcal{P}_{A:B} &= \frac{1}{2}(|\gamma_A| + |\gamma_B|) - |\boldsymbol{x}| - \frac{1}{8} - 2|\gamma_{\boldsymbol{AB}}|, \\ \mathcal{P}_{B:C} &= \frac{1}{2}(|\gamma_B| + |\gamma_C|) - |\boldsymbol{y}| - \frac{1}{8} - 2|\gamma_{\boldsymbol{BC}}|, \\ \mathcal{P}_{C:A} &= \frac{1}{2}(|\gamma_C| + |\gamma_A|) - |\boldsymbol{z}| - \frac{1}{8} - 2|\gamma_{\boldsymbol{AC}}|.\end{aligned} \tag{V.5}$$

Note that during three-mode BS mixing operation, both $|\gamma_{\boldsymbol{A}}| + |\gamma_{\boldsymbol{B}}| + 2|\boldsymbol{x}|$ and $|\gamma_{\boldsymbol{AB}}|$ are no longer symplectic invariants.

According to Eq. (8) of the main text, the left three-mode CNP is calculated as

$$\mathcal{P}_{A:BC}^{(3)} + \mathcal{P}_{B:AC}^{(3)} + \mathcal{P}_{C:AB}^{(3)} = 3(\frac{1}{32} - \frac{1}{8}\mathcal{I}_2^{(3)} + \frac{1}{2}\mathcal{I}_1^{(3)} - 2\mathcal{I}_0^{(3)}) + (|\boldsymbol{x}| + |\boldsymbol{y}| + |\boldsymbol{z}|) - 4(|\boldsymbol{M_x}| + |\boldsymbol{M_y}| + |\boldsymbol{M_z}|). \tag{V.6}$$

Substituting the above result into the expression of $\mathcal{P}$. The total CNP $\mathcal{P}$, calculated by adding single-mode, two-mode, and three-mode CNP are given by

$$\begin{aligned}\mathcal{P} =& \Big[\mathcal{P}_A^{(1)} + \mathcal{P}_B^{(1)} + \mathcal{P}_C^{(1)}\Big] + \Big[\mathcal{P}_{AB}^{(2)} + \mathcal{P}_{BC}^{(2)} + \mathcal{P}_{CA}^{(2)}\Big] + \Big[\mathcal{P}_{A:BC}^{(3)} + \mathcal{P}_{B:AC}^{(3)} + \mathcal{P}_{C:AB}^{(3)}\Big] \\ =& \Big[ - |\gamma_A| - |\gamma_B| - |\gamma_C| + \frac{1}{2}(\lambda_A + \Lambda_A + \lambda_B + \Lambda_B + \lambda_C + \Lambda_C) - \frac{3}{4}\Big] + \Big[(|\gamma_A| + |\gamma_B| + |\gamma_C|) - (|\boldsymbol{x}| + |\boldsymbol{y}| + |\boldsymbol{z}|) - \frac{3}{8} \\ & - 2(|\gamma_{\boldsymbol{AB}}| + |\gamma_{\boldsymbol{BC}}| + |\gamma_{\boldsymbol{AC}}|)\Big] + \Big[3(\frac{1}{32} - \frac{1}{8}\mathcal{I}_2^{(3)} + \frac{1}{2}\mathcal{I}_1^{(3)} - 2\mathcal{I}_0^{(3)}) + (|\boldsymbol{x}| + |\boldsymbol{y}| + |\boldsymbol{z}|) - 4(|\boldsymbol{M_x}| + |\boldsymbol{M_y}| + |\boldsymbol{M_z}|)\Big] \\ =& 3(\frac{1}{32} - \frac{1}{8}\mathcal{I}_2^{(3)} + \frac{1}{2}\mathcal{I}_1^{(3)} - 2\mathcal{I}_0^{(3)}) - \frac{3}{4} - \frac{3}{8} + \frac{1}{2}(\lambda_A + \Lambda_A + \lambda_B + \Lambda_B + \lambda_C + \Lambda_C) - 2(|\gamma_{\boldsymbol{AB}}| + |\gamma_{\boldsymbol{BC}}| + |\gamma_{\boldsymbol{AC}}|) \\ & - 4(|\boldsymbol{M_x}| + |\boldsymbol{M_y}| + |\boldsymbol{M_z}|) \\ =& -\frac{3}{8}\mathcal{I}_2^{(3)} - \frac{1}{2}\mathcal{I}_1^{(3)} - 6\mathcal{I}_0^{(3)} - \frac{33}{32} + \frac{1}{2}\bar{\Lambda}\end{aligned} \tag{V.7}$$

where $\bar{\Lambda} = \lambda_A + \Lambda_A + \lambda_B + \Lambda_B + \lambda_C + \Lambda_C$ is invariant during BS mixing operation.

## VI. Proof of theorem 2

Proof: Any pure Gaussian state can be generated using single-mode squeezing, two-mode squeezing, and two-mode beam-splitter mixing operations acting upon coherent states. As previously demonstrated, the total CNP, when considering both single-mode squeezed vacuum states and two-mode squeezed vacuum states, corresponds to the mean photon number of the

given state. It's important to note that the mixing operation is a linear optical transformation, ensuring that the total CNP remains invariant.


[1] M. O. Scully and M. S. Zubairy, *Quantum optics* (Cambridge University Press, Cambridge, England, 1997).
[2] C. T. Lee, Physical Review A **44**, R2775 (1991).
[3] A. Serafini, Physical Review Letters **96**, 110402 (2006).
[4] A. Serafini, *Quantum continuous variables: a primer of theoretical methods* (CRC press, 2023).
[5] V. I. Arnol'd, *Mathematical methods of classical mechanics 2nd. ed.*, Vol. 60 (Springer-Verlag, New York, 1989).
[6] G. Giedke, *Quantum information and continuous variable systems*, Ph.D. thesis, Institut für Theoretische Physik der Leopold-Franzens–Universität Innsbruck (2001).
[7] X.-B. Wang, T. Hiroshima, A. Tomita, and M. Hayashi, Physics Reports **448**, 1 (2007).
[8] R. Simon, Physical Review Letters **84**, 2726 (2000).
